# Supplementary material for: QuickCSG: Fast Arbitrary Boolean Combinations of N Solids
Source: arXiv:1706.01558 source file (2017-06-05)
Supplement: Supplementary file 1 [file appendix.tex]

\section{Finding the orientation of a partial mesh}
\label{sec:extremalappendix}

When splitting a kd-tree node, we need to find whether the splitting
plane is inside or outside a mesh, during the splitting pass. The orientation is
given by the normal of one facet, the ``extremal'' facet. This facet is the one closest and most parallel to the
splitting plane.
For example, for the mesh in
Figure~\ref{fig:meshorient}(a), if $v$ is the vertex with highest $z$
coordinate, then the normal of F0 gives the mesh orientation.
This is tricky because the mesh is possibly open, it may be cut during
the bounding box splits.

We want to find the extremal facet in one pass over the facets of the
mesh. During this pass, we keep track of the vertex with highest $z$
seen so far, $z_\mathrm{max}$. Then we intersect all the facets that
reach this $z_\mathrm{max}$ with plane \footnote{In practice, we set
$\varepsilon = 1$ and work with infinite facets} $ z = z_\mathrm{max} -
\varepsilon$, and project the extremal point $v$ on the plane as
$v'$. Each facet intersects as a segment.
Henceforth, we work in this
2D plane.

To find the extremal faacet, we consider the edge most
remote from $v'$. In Figure~\ref{fig:meshorient}(b), this is $e_{12}$,
its distance is $d_\mathrm{max}$. This leaves two possibilities for
the extremal facet: F1 or F2. In Figure~(b) both have the same
normal orientation, so it does not matter, but in figure~(c), their
orientations are different.

To distinguish between F1 and F2, we choose the one whose slope is
closest to orthogonal wrt. $(v', e_{12})$. For example, the slope for F1 is given by
\begin{equation}
s = \left| \frac{<(v' - e_{12})_\bot, e_{13} - e_{12}>} { ||v' - e_{12}|| . ||e_{13} - e_{12}||} \right|.
\end{equation}

In sum, the extremal facet is given by the maximum of the triplet $(z, d,
s)$. The triplets are compared lexicographically, ie. we compare $d$
values only if the $z$ values are the same. The current maximum of the
triplet and its associated normal vector can be be maintained in one
pass over the mesh facets. Since the triplets for different facets are computed in the same 
way from the vertex coordinates, they are exactly the same: there are no 
roundoff errors to take care of when testing for equality.

\begin{figure}
\includegraphics[width=\linewidth]{figs/extremal}
\caption{\label{fig:meshorient}
  Finding the mesh orientation in the positive $z$ direction. 
}
\end{figure}

\section{Computing corners from the vertex position}
\label{sec:cornersappendix}

In this section we detail how to find the half-edges connected to a
vertex $v$ known to belong to the result mesh
(function~\textsc{VertexCorners} in Algorithm~\ref{algo:csgfaces}). At
a time, we are interested only in the half-edges in one of the facets,
of the vertex. The input information is the mesh position of
the vertex and the facet id, the output a list of corners. The
notations are introduced in Section~\ref{sec:csgfaces}. Without 
loss of generality, we call F0 the input facet and F1, F2 the two other facets $v$ is the intersection of.

The bit vector $b$ of Equation~(\ref{eq:v1}), (\ref{eq:v2}) or
(\ref{eq:v3}) can be computed from the mesh position of vertex $v$. 
The corners are computed by bit pattern matching on $b$. In
practice $b$ is encoded in an integer, so this operation is 
very efficient.

We consider only the case $\Theta = 1$, ie. building the edges of the
output facets whose normal points into the same direction as the input
facet. The corners for the case $\Theta = -1$ can be obtained by
flipping $b$'s bits and by reverting the half-edges and their
order, ie. (F1+, $v$, F2-) becomes (F2+, $v$, F1-).

\subsection{Primary vertices}

In this case, vector $b$ of equation (\ref{eq:v1}) is $b=(b_1, b_2) = (0, 1)$.

Primary points are just copied to the output mesh, their corners are
the same as those of the input mesh, see
Figure~\ref{fig:corners}(a). The output corner is (F1+, $v$, F2+):
\begin{equation}
b = (0, 1) \rightarrow \textrm{(F1+, $v$, F2+)}.
\end{equation}
Note that for primitive vertices, there may be more that three facets
intersecting: in the figure, facets F1 and F2 are not adjacent.

\subsection{Double vertices}

A double point is the intersection of an edge with a facet. We will
distinguish the case where F0 is an incident facet of the edge and
when F0 is the facet the edge intersects with.

\subsubsection{Edge intersects with F0}

\newcommand{\nabu}{\bullet}

\newcommand{\quadrant}[4]{\rule{0pt}{1.7em}\begin{array}{|c|c|}
\hline
\makebox[0.7em][c]{$#1$} & \makebox[0.7em][c]{$#2$} \\
\hline
\makebox[0.7em][c]{$#3$} & \makebox[0.7em][c]{$#4$} \\
\hline
\end{array}}

We call F1 and F2 the facets of another mesh that F0 is intersecting
with, see Figure~\ref{fig:corners}(b)

In this case, there is a single possible corner, with two possible
orientations: (F1+, $v$, F2+) and (F2-, $v$, F1-). The orientation
encodes which side of the facet will be kept: respectively behind or
in front of F1 and F2 (as seen on the figure).

The choice depends on the values of the
CSG operation $f$ computed in the 4 quadrants of
Equation~(\ref{eq:v2}). If we note the 4 values in a $2\times2$ array with 
\begin{equation}
b=
\quadrant{b_1}{b_2}{b_3}{b_4}
\label{eq:twobytwo}
\end{equation}
ie. the fist line is for outside F0's mesh, and the second column
refers to the inside of F1 and F2's mesh. The $2\times2$ table is also drawn on
the figure.

Let's consider the part of the facet that is in front, as seen on the
figure. It exists if, outside of F1's mesh, F0 delimits an inside and
outside volume, ie. when:
\begin{equation}
\quadrant{0}{\nabu}{1}{\nabu} \rightarrow \textrm{(F2-, $v$, F1-)},
\label{eq:doubleA1}
\end{equation}
where $\nabu$ is a ``free'' bit, whose value does not matter. This covers the configurations:
\[
\quadrant{0}{0}{1}{0}, \quadrant{0}{1}{1}{1}, \quadrant{0}{1}{1}{0} \textrm{~(xor-style), and } 
\quadrant{0}{0}{1}{1} \textrm{:~(impossible)}
\]
The last one cannot occur because there would be no vertex there in the first place.
Similarly, for the corner behind F2: 
\begin{equation}
\quadrant{\nabu}{0}{\nabu}{1} \rightarrow \textrm{(F1+, $v$, F2+)}.
\label{eq:doubleA2}
\end{equation}
Note that the cases~(\ref{eq:doubleA1}) and~(\ref{eq:doubleA2}) are mutually exlusive because their
intersection is the impossible configuration.

\subsubsection{F0 is an incident facet of the edge}

We call F1 the other side of the edge and F2 the facet the edge
intersects with, see Figure~\ref{fig:corners}(b). There are two
orientations, depending on whether F1+ is  in the same
direction as F2's normal vector (left orientation) or the opposite
direction (right orientation). This can be determined from their dot product.

In both cases, either the corner in front or behind F2 is kept (as seen on the figure).
Using the same array notation as Equation~(\ref{eq:twobytwo}) where 
the fist line is for outside F0's mesh, and the second column
refers to the inside of F2's mesh (see the $2\times 2$ grids on the figure), 
this produces the following conditions:

\[
\begin{array}{ll}
\textrm{left} & 
\textrm{right} \\
\quadrant{0}{\nabu}{1}{\nabu} \rightarrow \textrm{(F1+, $v$, F2-)} & 
\quadrant{\nabu}{0}{\nabu}{1} \rightarrow \textrm{(F2+, $v$, F1+)} \\
\quadrant{\nabu}{0}{\nabu}{1} \rightarrow \textrm{(F1+, $v$, F2+)} & 
\quadrant{0}{\nabu}{1}{\nabu} \rightarrow \textrm{(F2-, $v$, F1+)} \\
\end{array}
\]

\begin{figure}
\hspace*{-5mm}
\begin{tabular}{|cc|}
\multicolumn{2}{c}{(a) primitive vertex}\\
\hline
\multicolumn{2}{|c|}{\includegraphics[scale=0.25]{figs/corners/primitive}} \\
\hline
\multicolumn{2}{c}{(b) double vertex}\\
\hline
\multicolumn{2}{|c|}{edge intersects F0}\\
\multicolumn{2}{|c|}{\includegraphics[scale=0.25]{figs/corners/doubleA2}} \\
\hline
\multicolumn{2}{|c|}{F0 incident to edge}\\
left  & right \\
\includegraphics[scale=0.25]{figs/corners/doubleB} & 
\includegraphics[scale=0.25]{figs/corners/doubleA} \\
\hline
\multicolumn{2}{c}{(c) triple vertex}\\
\hline
left  & right \\
\includegraphics[scale=0.25]{figs/corners/tripleA} &
\includegraphics[scale=0.25]{figs/corners/tripleB} \\
\hline
\end{tabular}
\caption{\label{fig:corners}
  Double and triple vertex configurations. The normal vector of each facet points
  outwards the mesh it belongs to.
}
\end{figure}

\subsection{Triple vertices}

Triple point also arrive in two possible orientations, depending on
whether the basis comprising their three normal vectors is left- or
right-handed, see Figure~\ref{fig:corners}(c).

We denote the 8 values of Equation~(\ref{eq:v3}) as 
\begin{equation}
b=
\begin{array}{|c|c||c|c|}
\hline
b_1 & b_2 & b_5 & b_6\\
\hline
b_3 & b_4 & b_7 & b_8 \\
\hline
\end{array},
\label{eq:twobyfour}
\end{equation}
where the two $2\times2$ sub-tables refer to the outside and inside of F0's
mesh, and the first row is for the outside of F1's mesh, and the
second and fourth column are for F2's inside.

\newcommand{\octant}[8]{\rule{0pt}{1.7em}\begin{array}{|c|c||c|c|}
\hline
\makebox[0.7em][c]{$#1$} & \makebox[0.7em][c]{$#2$} & \makebox[0.7em][c]{$#5$} & \makebox[0.7em][c]{$#6$} \\
\hline
\makebox[0.7em][c]{$#3$} & \makebox[0.7em][c]{$#4$} & \makebox[0.7em][c]{$#7$} & \makebox[0.7em][c]{$#8$} \\
\hline
\end{array}}

\newcommand{\nabuAI}{\alpha_1}
\newcommand{\nabuAO}{\alpha_0}
\newcommand{\nabuBI}{\beta_1}
\newcommand{\nabuBO}{\beta_0}
 
Let's consider the front corner in the ``left'' configuration. It exists in two cases:
\begin{itemize} %
\item concave corner (that covers 3/4 of the quadrant):
\begin{equation}
  \octant{\nabu}{0}{0}{0}{\nabu}{1}{1}{1} \rightarrow \textrm{(F1+, $v$, F2+)}
\end{equation}
\item convex corner (covers 1/4 of the quadrant):
\begin{equation}
  \octant{0}{\nabuAO}{\nabuBO}{\nabu}{1}{\nabuAI}{\nabuBI}{\nabu}  \rightarrow \textrm{(F2-, $v$, F1-)}
\end{equation}
where $(\nabuAO, \nabuAI, \nabuBO, \nabuBI)$ are free bits, that verify the additional constraint that
  $(b_2, b_6) = (\nabuAO, \nabuAI) \ne (0, 1)$ and $(b_3,b_7) = (\nabuBO, \nabuBI)  \ne (0, 1)$. This is required for  edges
  F2- and F1- to exist. 
\end{itemize}

The complete set of configurations can be obtained by rotating around the vertical axis:
\[
\begin{array}{ll}
\textrm{left} & \textrm{right} \\
\octant{\nabu}{0}{0}{0}{\nabu}{1}{1}{1} \rightarrow \textrm{(F1+, $v$, F2+)} & 
\octant{0}{\nabu}{0}{0}{1}{\nabu}{1}{1} \rightarrow \textrm{(F1+, $v$, F2-)} \\
\octant{0}{\nabuAO}{\nabuBO}{\nabu}{1}{\nabuAI}{\nabuBI}{\nabu} \rightarrow \textrm{(F2-, $v$, F1-)} & 
\octant{\nabuAO}{0}{\nabu}{\nabuBO}{\nabuAI}{1}{\nabu}{\nabuBI} \rightarrow \textrm{(F2+, $v$, F1-)} \\

\octant{0}{0}{\nabu}{0}{1}{1}{\nabu}{1} \rightarrow \textrm{(F2+, $v$, F1-)} & 
\octant{\nabu}{0}{0}{0}{\nabu}{1}{1}{1} \rightarrow \textrm{(F2+, $v$, F1+)} \\
\octant{\nabuAO}{\nabu}{0}{\nabuBO}{\nabuAI}{\nabu}{1}{\nabuBI} \rightarrow \textrm{(F1+, $v$, F2-)} &
\octant{0}{\nabuBO}{\nabuAO}{\nabu}{1}{\nabuBI}{\nabuAI}{\nabu} \rightarrow \textrm{(F1-, $v$, F2-)}\\

\octant{0}{0}{0}{\nabu}{1}{1}{1}{\nabu} \rightarrow  \textrm{(F1-, $v$, F2-)} &
\octant{0}{0}{\nabu}{0}{1}{1}{\nabu}{1} \rightarrow  \textrm{(F1-, $v$, F2+)}\\
\octant{\nabu}{\nabuBO}{\nabuAO}{0}{\nabu}{\nabuBI}{\nabuAI}{1} \rightarrow  \textrm{(F2+, $v$, F1+)} &
\octant{\nabuBO}{\nabu}{0}{\nabuAO}{\nabuBI}{\nabu}{1}{\nabuAI} \rightarrow  \textrm{(F2-, $v$, F1+)}\\

\octant{0}{\nabu}{0}{0}{1}{\nabu}{1}{1} \rightarrow  \textrm{(F2-, $v$, F1+)} &
\octant{0}{0}{0}{\nabu}{1}{1}{1}{\nabu} \rightarrow  \textrm{(F2-, $v$, F1-)} \\
\octant{\nabuBO}{0}{\nabu}{\nabuAO}{\nabuBI}{1}{\nabu}{\nabuAI} \rightarrow  \textrm{(F1-, $v$, F2+)} &
\octant{\nabu}{\nabuAO}{\nabuBO}{0}{\nabu}{\nabuAI}{\nabuBI}{1} \rightarrow  \textrm{(F1+, $v$, F2+)}
\\
\end{array}
\]
At most two of those configurations can be active simultaneously, when
two convex corners are symmetric wrt. $v$, which occurs in xor-style
configurations. 
